# Supplementary material for: Observation of the sling effect
Source: arXiv:1312.2901 source file (2014-01-09)
Supplement: Supplementary file 1 [file Bewley.etal.sling.paper.supplementary.information.pdf]

# Observation of the sling effect

**Gregory P. Bewley**[1]

**Ewe-Wei Saw**[1]

**Eberhard Bodenschatz**[1,2]

[1]Max Planck Institute for Dynamics and Self-Organization, 37077 Göttingen, Germany

[2]Laboratory of Atomic and Solid State Physics and Sibley School of Mechanical and Aerospace Engineering, Cornell University, Ithaca, NY 14853, USA

E-mail: `gregory.bewley@ds.mpg.de`

## 1. Soccer-ball turbulence

We summarize here the main features of the apparatus and of the flow, and the differences between the present apparatus and the one of Chang et al. [1]. As seen in Fig. 1, the apparatus consisted of an acrylic shell with an inner diameter of 1 m, which contained air at standard temperature and pressure. Thirty-two loudspeakers were attached to the shell. Their positions corresponded to the centers of the faces of a truncated icosahedron, which is the shape of a traditional soccer ball. The loudspeakers were woofers (Visaton WS 17 E), were rated for 60 W, and had diameters of 17 cm. They pushed and pulled air through conical nozzles with opening angles of 30°, heights of 3.5 cm and orifice-diameters of 6 cm. This pushing and pulling of the air formed jets, which pointed toward the centre of the chamber where they interacted with each other [2]. The jets had the same strength, so that the turbulence was approximately isotropic within 50 mm of the centre of the sphere.

The Reynolds number, $R_\lambda = u'\lambda/\nu$ was about 170, where $u'$ is the RMS of the turbulent velocity fluctuations in a given direction, $\lambda$ is the Taylor scale, and $\nu$ is the viscosity of the fluid [3]. We determined $\lambda$ from the isotropic relationship $\lambda = (15\nu u'^2/\epsilon)^{1/2}$, where $\epsilon$ is the kinetic energy dissipation rate per unit mass of the turbulence. We determined $\epsilon$, in turn, from the dissipation-range scaling of the longitudinal second-order structure functions: $\langle((\mathbf{v}(\mathbf{x}+\mathbf{r},t) - \mathbf{v}(\mathbf{x},t)) \cdot \mathbf{r}(t)/r)^2\rangle = (\epsilon/15\nu)r^2$, where $r$ is the length of the separation vector $\mathbf{r}$. The 15% uncertainty we report in $\epsilon$ captures the deviations of the data from the square power law within the range of scales $1 < r/\eta < 5$.

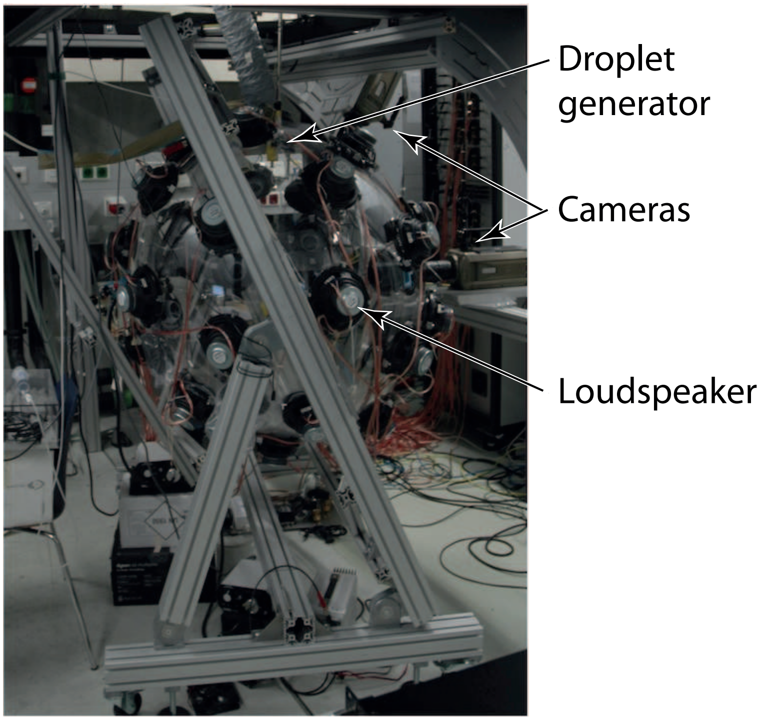


**Figure 1.** The experimental setup. The sphere in the middle with the loudspeakers attached to it is the turbulence chamber. In the upper right are the two high speed cameras, which point toward the centre of the sphere. Directly opposite each camera is a light source, which is difficult to distinguish in this picture. The particle generator is mounted beneath the top wall of the soccer-ball, and can be seen magnified in Fig. 2.

## 2. Particle generation

Particles with a bimodal size distribution were generated by a spinning disk [4]. Our design was similar to the one of Philipson [5], and consisted of a circular disc coupled to a turbine driven by pressurized air. Our turbine spun at up to 100,000 rotations per minute. As shown in Fig. 2, the circular disc was made of stainless steel, and had diameter of 2 cm with disc edge cut at 45°. The surface and edge of the disc were smooth.

Liquid with low surface tension, 40% ethanol by volume in water, was pumped at about 1 milliliter per minute to the centre of the disc through a syringe needle. The technique works by centrifuging the liquid toward the edge, where a Rayleigh-Taylor instability forms regularly spaced bulges in the liquid. When the centrifugal acceleration is high enough relative to the surface tension, each bulge ejects a primary drop followed by several smaller satellite drops. The advantage of this method is that it produces particles at a high rate, relative to other methods, and the particles have narrow size distributions.

The mean sizes of the primary and satellite particles are tunable by adjusting the rotation rate of the disc. In our experiment, we produced primary and satellites particles with mean diameters of 19.4 $\mu m$ and 6.8 $\mu m$, respectively. For both the primary and

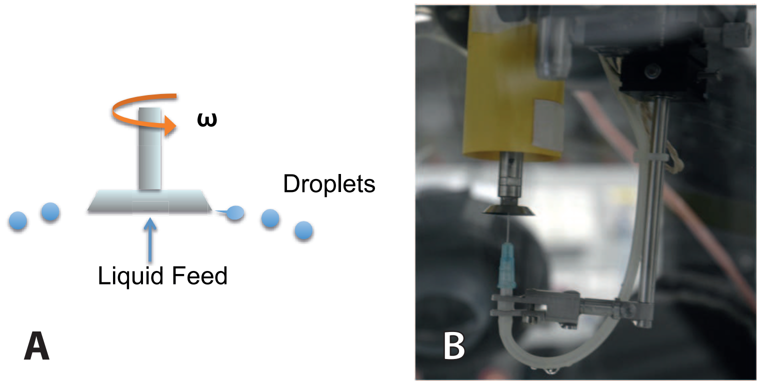


**Figure 2.** (A) A schematic of the spinning disc particle generator. A liquid wets the disc surface and is drawn toward its edge by centrifugal forces. A liquid instability causes particles to be ejected from the edge of the disc. (B) A picture of the particle generator. Visible are the disc and the syringe needle that supplied liquid to the centre of the disc. The air turbine is shrouded by the yellow cylinder.

satellite particles, the standard deviation in the size of the particles was about 22% of their mean diameters.

## 3. Particle imaging

Nishino et al. [6] and Lee et al. [7] demonstrate the utility of shadow-imaging in particle tracking and in particle sizing, while Ouellette et al. [8] describes how to reconstruct stereoscopically the three-dimensional (3D) particle positions from two (or more) images. In this section, we describe the techniques of particle imaging, sizing, and location that were particular to our experiment in which the particles were particles.

The cameras were two Vision Research Phantom V640 cameras, which were focussed onto the same volume. The angle included by the lines of sight of the two cameras was about 60°. We used Nikon Micro-Nikkor 200 mm lenses in combination with teleconverters as long-range microscope objectives. The magnification in the focal volume of the cameras was 3.3.

The light sources were fibre-guided halogen lamps from Thorlabs. The light was focused by lenses into an approximately $1\,cm^3$ volume of interest in the centre of the turbulence chamber. The light shown through the volume of interest and directly into the cameras. In the focal volume of the cameras, the particles acted as lenses that scattered light so that the particles appeared as dark spots in the images.

To find the 3D positions of the particles in real space, we combined the two-dimensional coordinates of the particles' images in two cameras [8]. We defined the particle positions in an image as the centers of mass of contiguous regions of pixels whose intensities were below a certain threshold. The accuracy in determining the 3D particle positions was approximately $0.2\,\mu m$ along the axis bisecting the two cameras' lines of sight, and about $0.1\,\mu m$ in the directions transverse to this axis.

We measured the areas of the particle shadows to size the particles. The areas

were equal to the number of pixels below a certain threshold. particles were considered large if their area was greater than 25 pixels, and small otherwise. By this method, the shadow diameters of the large particles were consistently about 1.4 times larger than the actual diameters of the particles. The factor was 1.9 for the small particles. These factors were determined by imaging 6, 10, and 20 micron polymer microspheres. After correction for the bias, the two populations of particles had mean diameters of 19.4 $\mu m$ and 6.8 $\mu m$. The uncertainty in determining the mean was about 4% for the large particles and 10% for the small ones.

## 4. Particle tracking

We briefly describe here how we dealt with particular tracking issues. Tracking conflicts arose when two tracks competed for the same particle [8]. In these cases, the particle was not assigned to either track. The tracks were then assigned a virtual particle position by a predictive algorithm, and the tracking continued in the next frame. Tracks that encountered to too many conflicts sequentially were terminated.

Additional tracking ambiguities arose when two particles and the lines of sight of the cameras lay in a plane [9]. This scenario can result in the artificial production by the stereoscopic matching algorithm of two phantom particles. In order to eliminate these spurious particles, we tracked only those particles that had a unique image in each camera. That is, we discarded 3D particle positions that had a common particle image in any camera. This filtering necessarily resulted in the loss of good data, but had the advantage of introducing no spurious data.

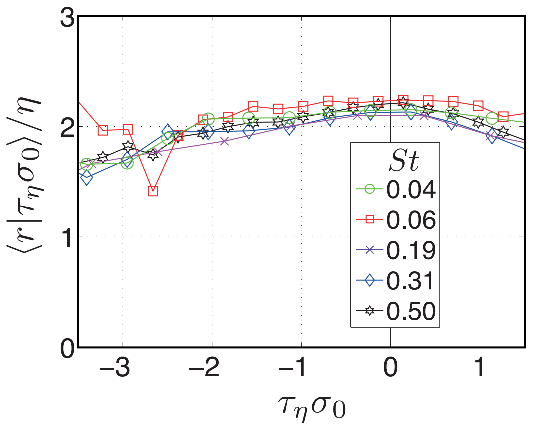


**Figure 3.** The mean separation between particles conditioned on the particle velocity gradient. The gradients are normalized by the turbulence time scale, $\tau_\eta$.

## 5. Experimental protocol

The data were taken in three runs, during which the turbulence had different dissipation rates. We produced the different dissipation rates by adjusting the amplitudes of the

loudspeaker vibrations. For each dissipation rate, the experiment was repeated many times, because the memory of the cameras was not large enough to collect sufficient data in a single realization. The memory was large enough for 9 s of data under the conditions described in the sections above.

Because two sizes of particles were present at the same time, each run produced data with two different Stokes numbers. We do not show the small-particle data for the lowest dissipation rate case, because it agrees with the other data and only clutters the presentation. The dissipation rates were measured for each run using the lower Stokes number data in each case, according to the method described above.

At the beginning of each run, the particle generator was run for several minutes in order to saturate the air in the turbulence chamber with alcohol and water vapor. This prevented particle evaporation. We then waited until the average number density of the particles was about 1000 $cm^{-3}$, with a variation of about 50% from run to run. Over the duration of each movie, the particle number density decreased by up to 20% due to deposition on chamber walls. This however, is irrelevant to the analysis and conclusion of current study.

Once the chamber was seeded with particles, we turned on the turbulence and waited about 5 s before acquiring data. The procedure was repeated every half hour, which is approximately the time needed to recover the newly acquired data from the cameras. A total of about 600, 700 and 1200 s of data were acquired in each run, in order of increasing dissipation rate. This corresponded to about $10^4$ eddy turn over times in each case.

## 6. Distance between particles

We measured gradients by finite differences made between particles separated by up to $3\eta$. In Fig. 3, we show the mean separation between particles as a function of the velocity gradient between the particles. The mean separation was about $2\eta$, which was about 20 times larger than the diameter of the large particles and 60 times larger than the small ones. The most probable separation was closer to $3\eta$ than 0 since the chance of finding particles at some distance increases approximately as the square of this distance. When the gradients were sharp, the particles tended to be closer together, being about 25% closer when $\tau_\eta\sigma_0$ was -3 than when it was 0. The amplitude of the effect was the same for all Stokes numbers, which suggests that it was not caused by particle inertia, and may have been due to sampling bias.

## 7. The role of gravity

Gravity could affect our measurements in two ways. The direction of gravity could both break the rotational symmetry of the dynamics, and produce an offset in the relative velocities between particles. The latter effect is due to the small differences in sizes between the particles, which causes some particles to settle faster than others. If we

imagine the worst-case, and unrealistic, scenario in which only one particle in each pair is settling, it is easy to calculate the offset to $\tau_p \sigma_0$. The offset is $\tau_p^2 g/r$, since the settling velocity of one particle is $\tau_p g$. This offset would shift the data to the left or to the right in Figs. 3 and 4 of the manuscript, depending on the direction of gravity relative to the separation vector between the particles. In our experiment, $\tau_p^2 g/r = 0.03$, which is small relative to $\tau_p \sigma_0 \sim 1$. Note in addition that our data are averages made between particles aligned at all angles with respect to gravity, so that gravitational offsets probably average out.

The influence of gravity can also be parameterized by the ratio of the settling velocity to the Kolmogorov velocity. Considering the large (20 micron) particles first, this ratio decreased from 0.21 to 0.13 as the Stokes number increased from 0.19 to 0.5. For the small particles, the ratio was decreased from 0.026 to 0.020 as the Stokes number decreased from 0.06 to 0.04. This can be understood intuitively to mean that the particles fell through the smallest turbulent eddies more slowly than the characteristic velocities of the eddies themselves.

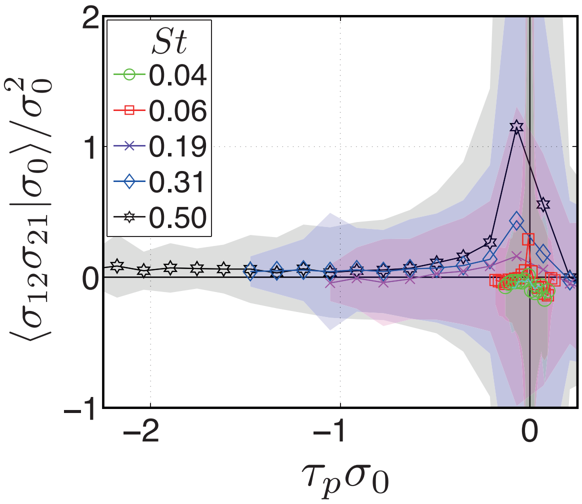


**Figure 4.** The transverse gradient correlations, $\langle \sigma_{12}\sigma_{21}|\sigma_0\rangle$, appear in the conditionally averaged dynamical equations for the longitudinal gradients. The square of the longitudinal gradients, $\sigma_0^2$, drives slings, and we show here that for large values of $|\tau_p \sigma_0|$, the transverse gradients were not large enough to counteract the effect of $\sigma_0^2$. Not only this, but they were slightly positive, which tends to enhance the sling effect. The shaded regions enclose data within one standard deviation of the mean, as in Fig. 4A of the main text.

## 8. Gradient correlation calculation

We measured the cross terms introduced above with a third particle. That is, we used triads of particles to estimate the transverse velocity gradient correlations. For each triad, the third particle was selected so that the separation vector to it, $\mathbf{r}_\perp$, was approximately perpendicular to $\mathbf{r}$, the separation vector between the first two particles.

It follows that

$$\sigma_{12}\sigma_{21} \approx \left(\frac{\delta\mathbf{v}\cdot\hat{\mathbf{r}}_\perp}{r}\right)\left(\frac{\delta\mathbf{v}_\perp\cdot\hat{\mathbf{r}}}{r_\perp}\right), \qquad (1)$$

where $\delta\mathbf{v} = \mathbf{v}(\mathbf{x}+\mathbf{r})-\mathbf{v}(\mathbf{x})$ as before, and $\delta\mathbf{v}_\perp = \mathbf{v}(\mathbf{x}+\mathbf{r}_\perp)-\mathbf{v}(\mathbf{x})$ is the velocity difference to the third particle. Note that the conditionally averaged quantities $\langle\sigma_{12}\sigma_{21}|\sigma_0\rangle$ and $\langle\sigma_{13}\sigma_{31}|\sigma_0\rangle$ have the same expectation value because the flow was isotropic.

Figure 4 shows these correlations as a fraction of the term that drive the sling, $\sigma_0^2$, or $\langle\sigma_{12}\sigma_{21}|\sigma_0\rangle/\sigma_0^2$. For $|\tau_p\sigma_0| > 1$, the correlations were very small, and for our purposes negligible. We emphasize that slings are associated with longitudinal compressive strains, and not with rotations.

## References


[1] Chang K, Bewley GP and Bodenschatz E 2012 Experimental study of the influence of anisotropy on the inertial scales of turbulence *J. Fluid Mech.* **692** 464–481

[2] Hwang W and Eaton JK 2004 Creating homogeneous and isotropic turbulence without a mean flow *Exp. Fluids* **36** 444–454

[3] Frisch U 1995 *Turbulence: The Legacy of A.N. Kolmogorov* (Cambridge University Press)

[4] Walton WH and Prewett WC 1949 The production of sprays and mists of uniform drop size by means of spinning disc type sprayers *Proc. Phys. Soc. B* **62** 341–350

[5] Philipson K 1973 On the production of monodisperse particles with a spinning disc *Aerosol Sci.* **4** 51–57

[6] Nishino K, Kato H and Torii K 2000 Stereo imaging for simultaneous measurement of size and velocity of particles in dispersed two-phase flow *Meas. Sci. Technol.* **11** 633–645

[7] Lee C, Wu CH and Hoopes JA 2009 Simultaneous particle size and concentration measurements using a back-lighted particle imaging system *Flow Meas. and Instrum.* **20** 189–199

[8] Ouellette NT, Xu H, Bourgoin M and Bodenschatz E 2006 An experimental study of turbulent relative dispersion models *New J. Phys.* **8** 109

[9] Maas HG, Gruen A and Papantoniou D 1993 Particle tracking velocimetry in three-dimensional flows, part 1. photogrammetric determination of particle coordinates *Exp. Fluids* **15** 133–146
